# Supplementary material for: Exploring Set Similarity for Dense Self-supervised Representation Learning
Source: arXiv:2107.08712 source file (2022-03-14)
Supplement: Supplementary file 2 [file supplementary.tex]

% !TEX root = ../main.tex
\section{Appendix}

\subsection{COCO 2$\times$ schedule fine-tuning}

\myparagraph{Implementation.}
Following \cite{he2020momentum}, we utilize a Mask-RCNN \cite{he2017mask} (Keypoint-RCNN \cite{wu2019detectron2}) with FPN \cite{lin2017feature} as our base model and add new Batch Normalization layers before the FPN.
All Batch Normalization layers are synchronized across all devices.
We fine-tune the model with the standard $2\times$ schedule (\textasciitilde24 epochs) \cite{wu2019detectron2} for three tasks, object detection, instance segmentation, and keypoint detection.
Average Precision on bounding boxes (AP$^{b}$), masks (AP$^{m}$), and keypoints (AP$^{kp}$) are adopted as our metrics, which are the same with \cite{he2020momentum}.

\myparagraph{Main results.}
As illustrated in Table~\ref{tab:coco_det_ins_sup}, our method improves over the MoCo-v2 baseline \cite{he2020momentum} under both box and mask metrics, surpassing the supervised pretraining baseline.
Compared with the recently proposed DenseCL \cite{wang2020DenseCL} and PixPro \cite{xie2020propagate}, SetSim outperforms them on three tasks with the standard $1\times$ and $2\times$ schedules, which strongly demonstrates the effectiveness of our method.

% COCO detection & instance
\begin{table}[h]
    \setlength{\belowcaptionskip}{2.7pt}
    \begin{center}
    \caption{\textbf{Comparisons with the state-of-the-art approaches on COCO object detection, instance segmentation and keypoint detection.} 
    All methods are fine-tuned on \texttt{train2017} with 2$\times$ schedules and evaluated on \texttt{val2017}. 
    A Mask-RCNN (R50-FPN) \cite{he2017mask,wu2019detectron2} is adopted for all methods. 
    Average precision on bounding-boxes (AP$^{b}$), masks (AP$^{m}$) and keypoint (AP$^{kp}$) are used as benchmark metrics. 
    Following \cite{he2020momentum}, We fine-tune all methods with their official pretrained weights, ensuring a fair comparison.}
    \setlength{\tabcolsep}{2mm}{
    \begin{tabular}{l|ccc|ccc|ccc}
        \toprule[1.2pt]
        \multirow{2}{*}{Method} & \multicolumn{3}{c|}{Object Det.} & \multicolumn{3}{c|}{Instance Seg.} & \multicolumn{3}{c}{Keypoint Det.} \\
        \cline{2-10}
        ~ & AP$^{b}$ & AP$^{b}_{50}$ & AP$^{b}_{75}$ & AP$^{m}$ & AP$^{m}_{50}$ & AP$^{m}_{75}$ & AP$^{kp}$ & AP$^{kp}_{50}$ & AP$^{kp}_{75}$ \\
        \midrule[1.2pt]
        \textcolor{gray}{Random init.}         & \textcolor{gray}{36.7} & \textcolor{gray}{56.7} & \textcolor{gray}{40.0} & \textcolor{gray}{33.7} & \textcolor{gray}{53.8} & \textcolor{gray}{35.9} & \textcolor{gray}{65.4} & \textcolor{gray}{86.8} & \textcolor{gray}{71.9} \\ 
        IN-1K sup.                             & 40.6 & 61.3 & 44.4 & 36.8 & 58.1 & 39.5 & 65.7 & 87.0 & 72.0 \\
        \midrule
        MoCo-v1 \cite{he2020momentum}         & 40.3 & 61.0 & 43.9 & 36.5 & 57.9 & 39.0 & 66.4 & 87.3 & 61.7 \\
        MoCo-v2 \cite{chen2020improved}       & 40.8 & 61.3 & 44.3 & 36.9 & 58.5 & 39.5 & 66.9 & 87.7 & 72.9 \\
        DenseCL \cite{wang2020DenseCL}        & 41.2 & 61.8 & 44.9 & 37.3 & 58.8 & 40.2 & 67.2 & 87.5 & 73.4 \\
        PixPro \cite{xie2020propagate}        & 41.5 & 61.9 & 45.5 & 37.4 & 58.9 & 40.3 & 67.1 & 88.1 & 73.3 \\
        \midrule
        SetSim                                 & \textbf{41.6} & \textbf{62.4} & \textbf{45.9} & \textbf{37.7} & \textbf{59.4} & \textbf{40.6} & \textbf{67.4} & \textbf{88.1} & \textbf{73.4} \\
        \bottomrule[1.2pt]
    \end{tabular}
    \label{tab:coco_det_ins_sup}}
    \end{center}
\end{table}

\subsection{ImageNet Linear Evaluation}
\myparagraph{Implementation.}
Following a standard protocol \cite{he2020momentum,chen2020improved}, given a 200-epoch pretraining, we train a supervised linear classifier on frozen features extracted from ResNet's global average pooling layer.
The linear classifier adopts $lr=30$ with a cosine decay schedule for 90 epochs, $weight\,decay=0$, $momentum=0.9$, and $batch\,size=256$ with a SGD optimizer.
During testing, we evaluate the model on the center 224$\times$224 crop in the validation set.

\myparagraph{Main Results.}
Although our SetSim achieves significant improvements over the MoCo-v2 baseline on a series of dense prediction tasks,
the classification accuracy of our method is 2.1\% lower than MoCo-v2 (67.4\% \textit{v.s.} 69.5\%) at 200-epoch pretraining.
This phenomenon demonstrates that exploring dense representation is not necessary to image-level prediction tasks.
This is in accordance to a similar observation reported by \cite{chen2020simple}, where linear classification accuracy is not monotonically related to transfer performance in dense prediction tasks.
To this end, we validate the particular effectiveness of dense self-supervised representation learning for dense prediction tasks.

\subsection{Visualization on Downstream tasks}

\begin{figure}[h]
    \begin{center}
        \includegraphics[scale=0.45]{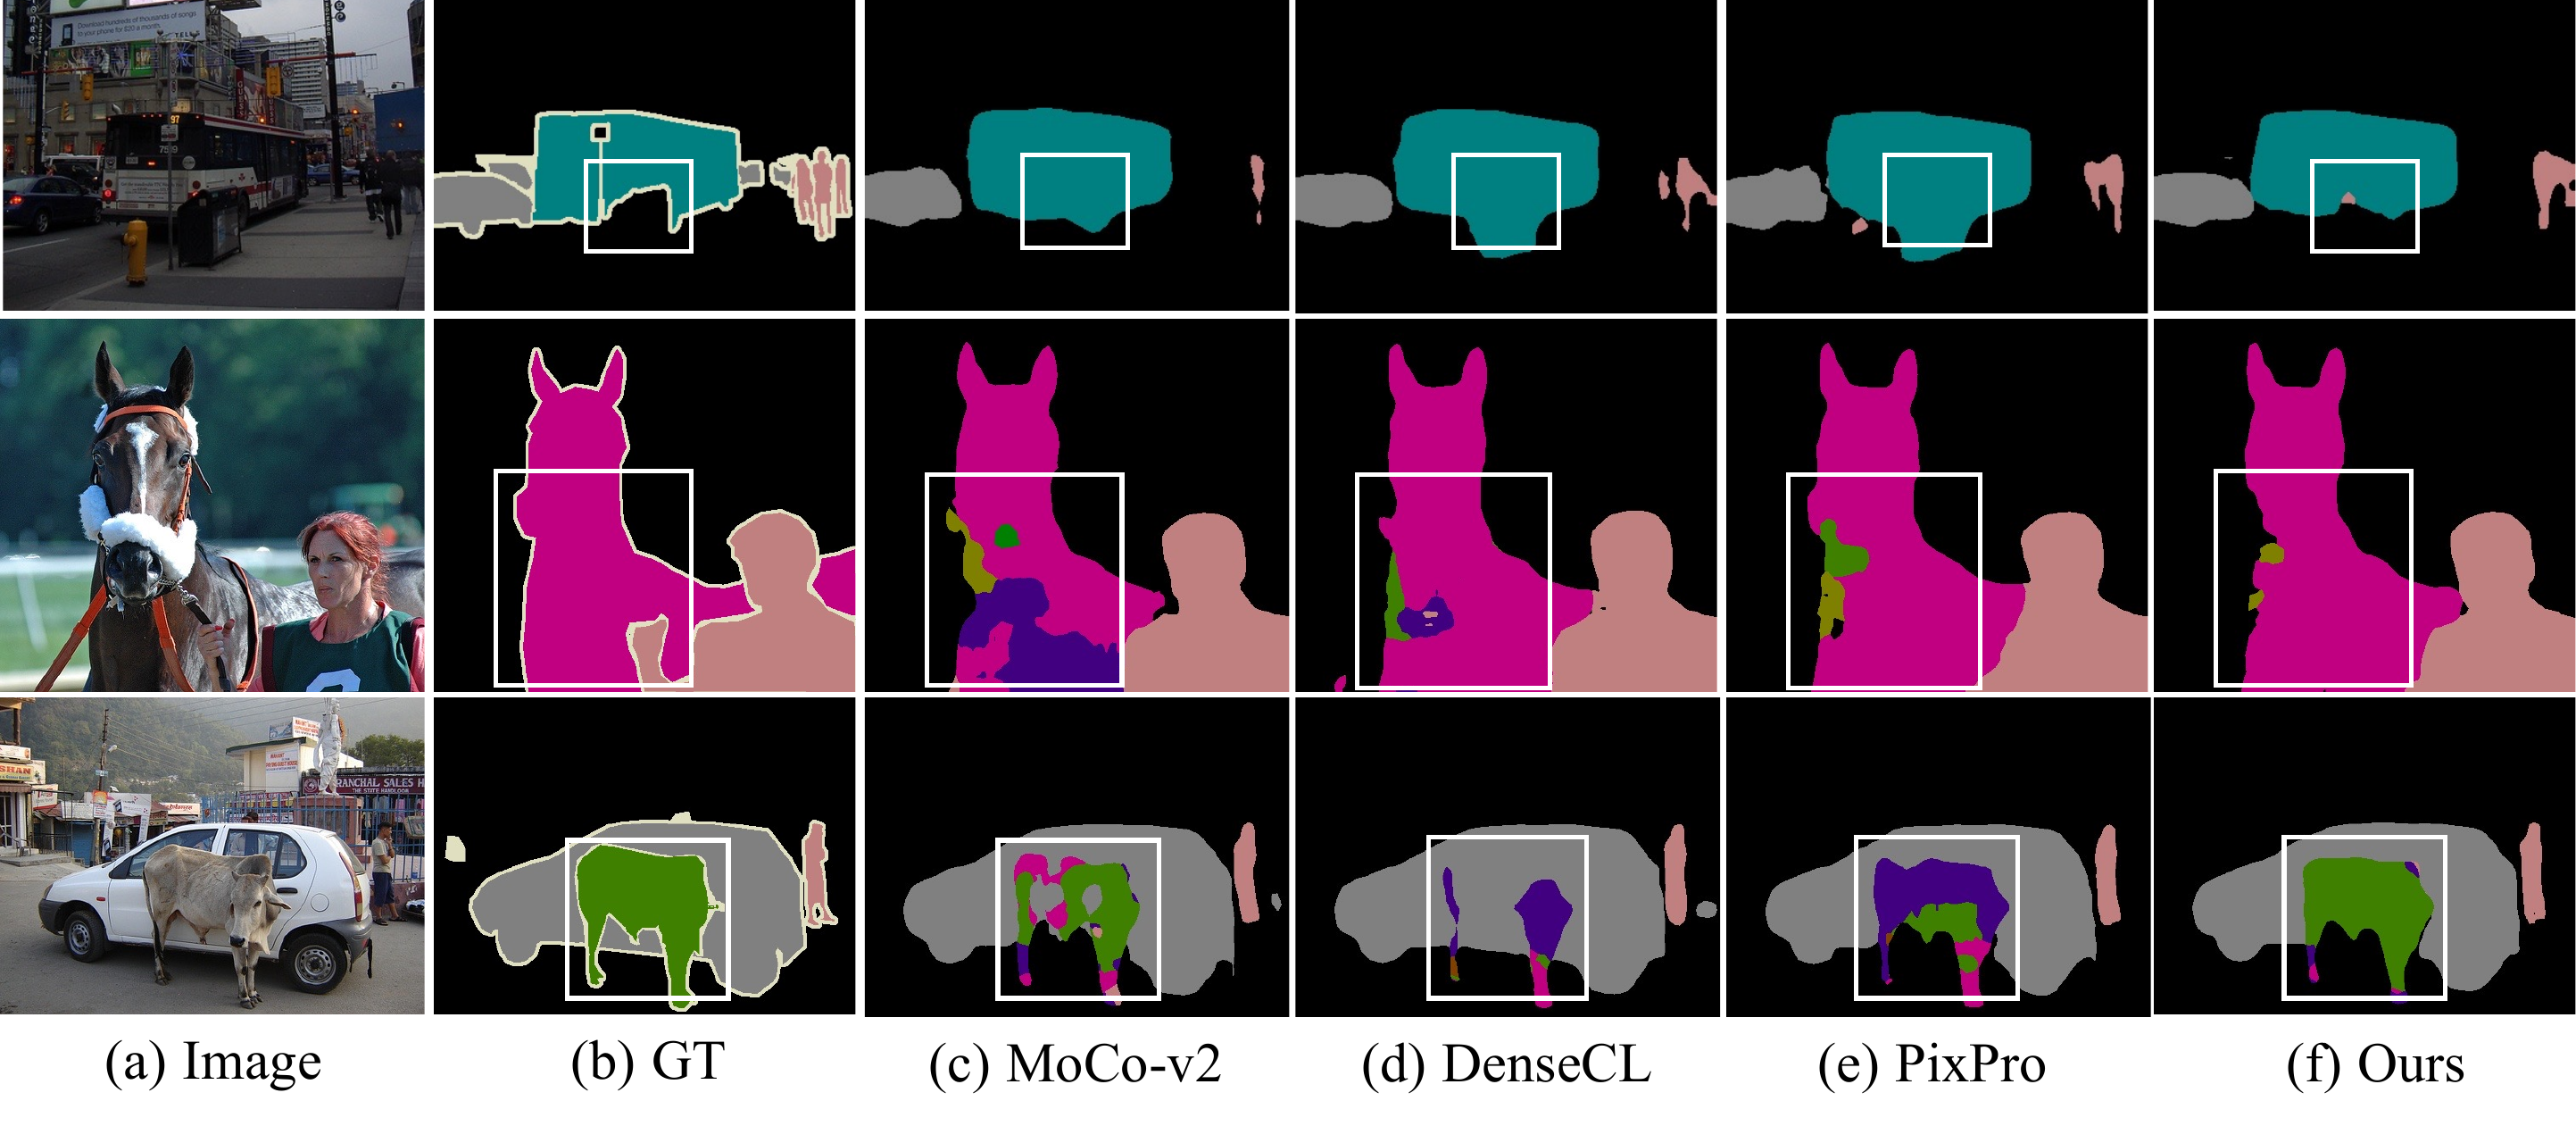}
        \caption{\textbf{Visualization results on PASCAL VOC object segmentation.}
        (\textit{Best viewed in color.})}
    \label{fig:voc_seg} 
    \end{center}
\end{figure}
\begin{figure}[h]
    \begin{center}
        \includegraphics[scale=0.45]{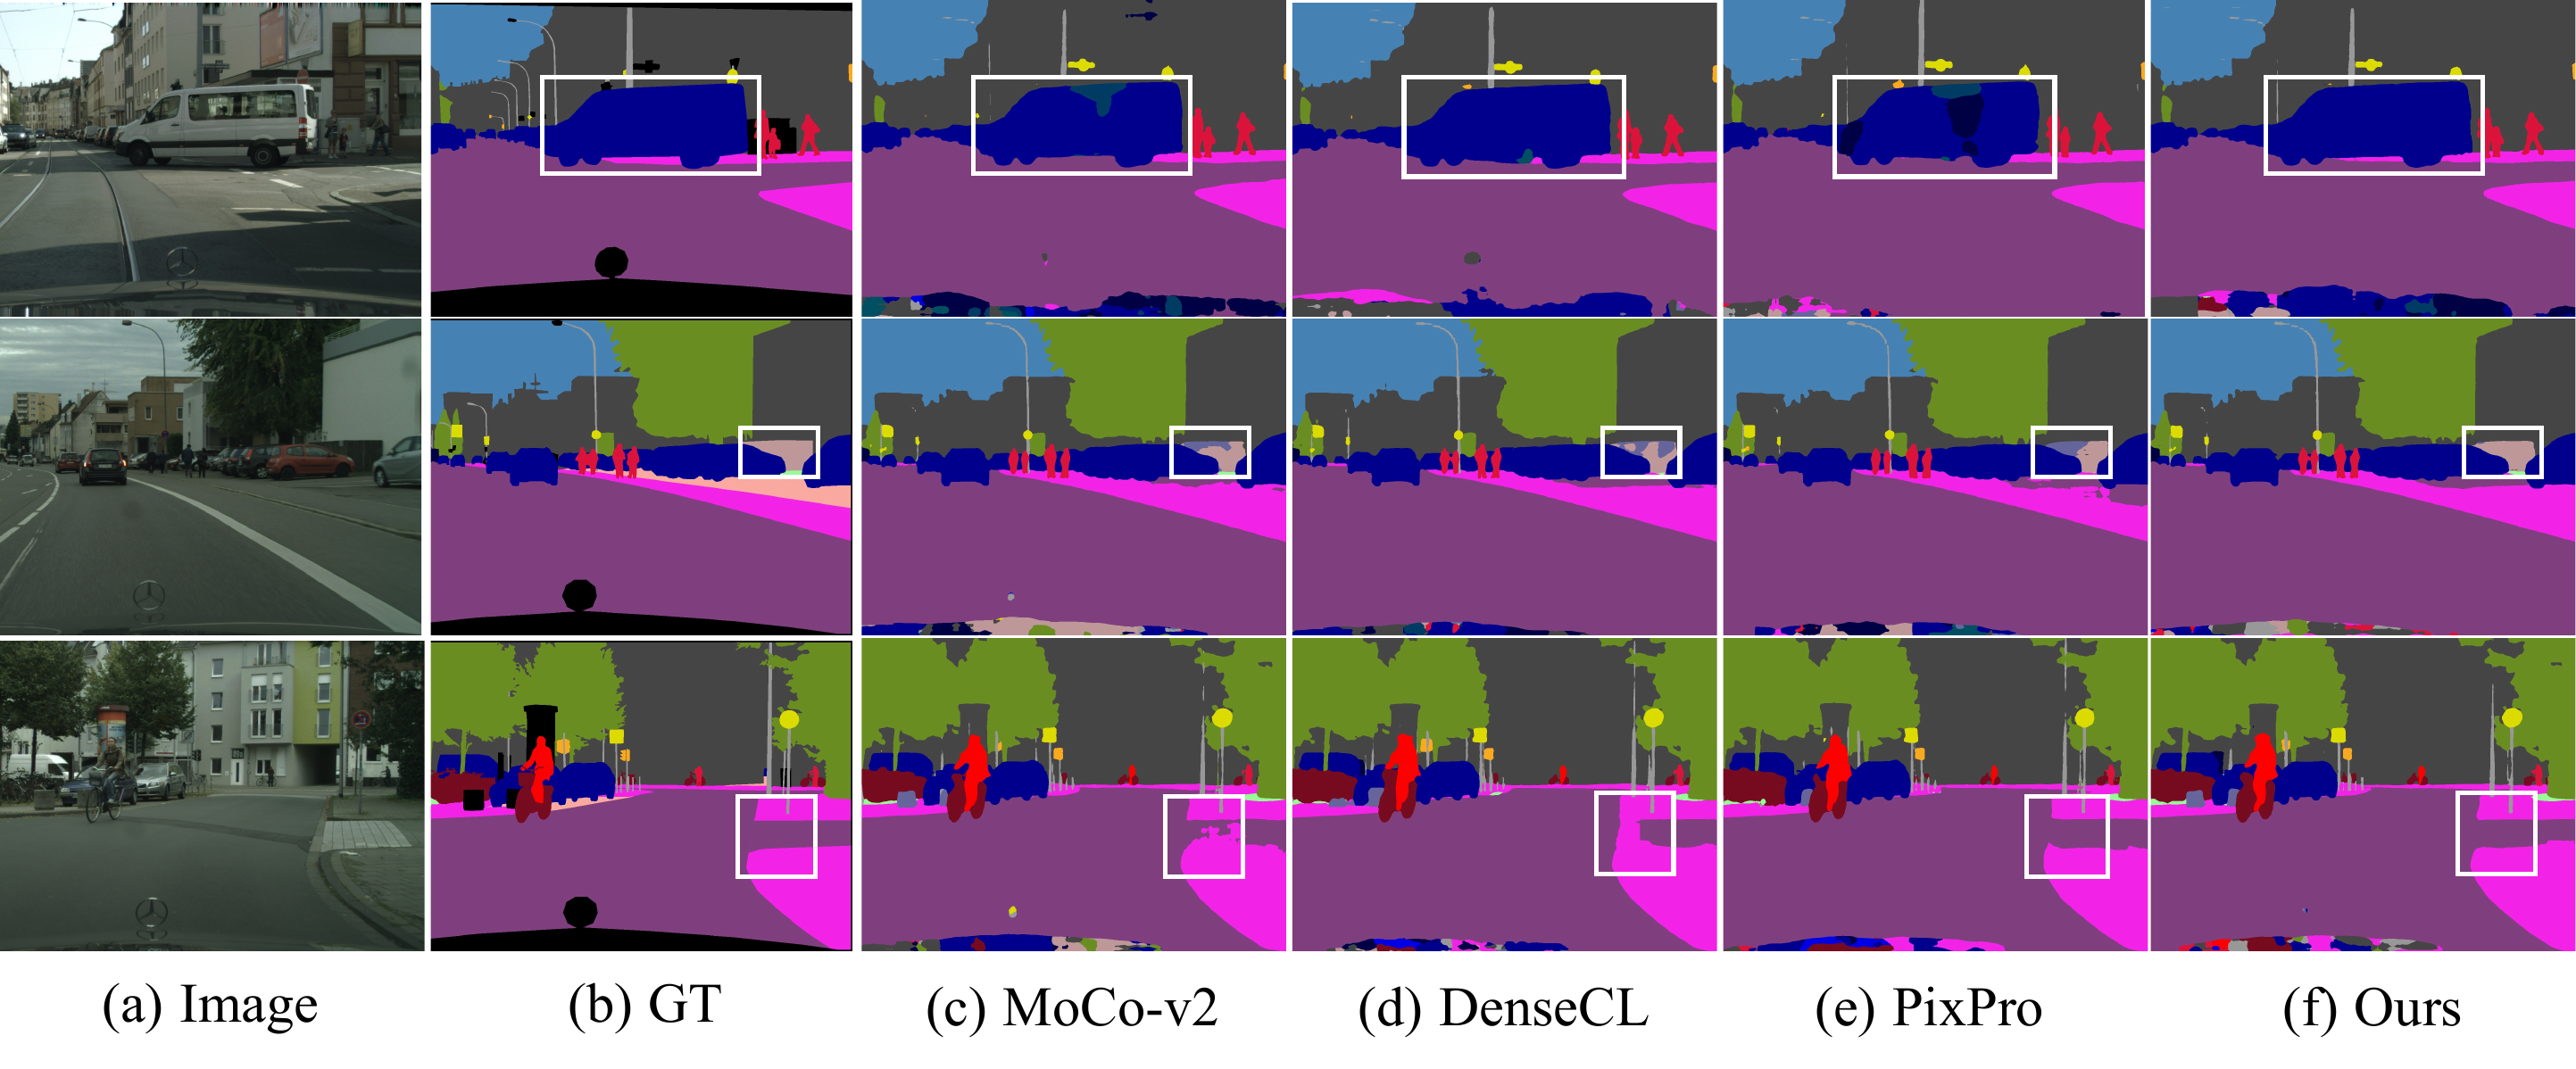}
        \caption{\textbf{Visualization results on Cityscapes semantic segmentation.}
        (\textit{Best viewed in color.})}
    \label{fig:citys_seg} 
    \end{center}
\end{figure}
\begin{figure}[h]
    \begin{center}
        \includegraphics[scale=0.45]{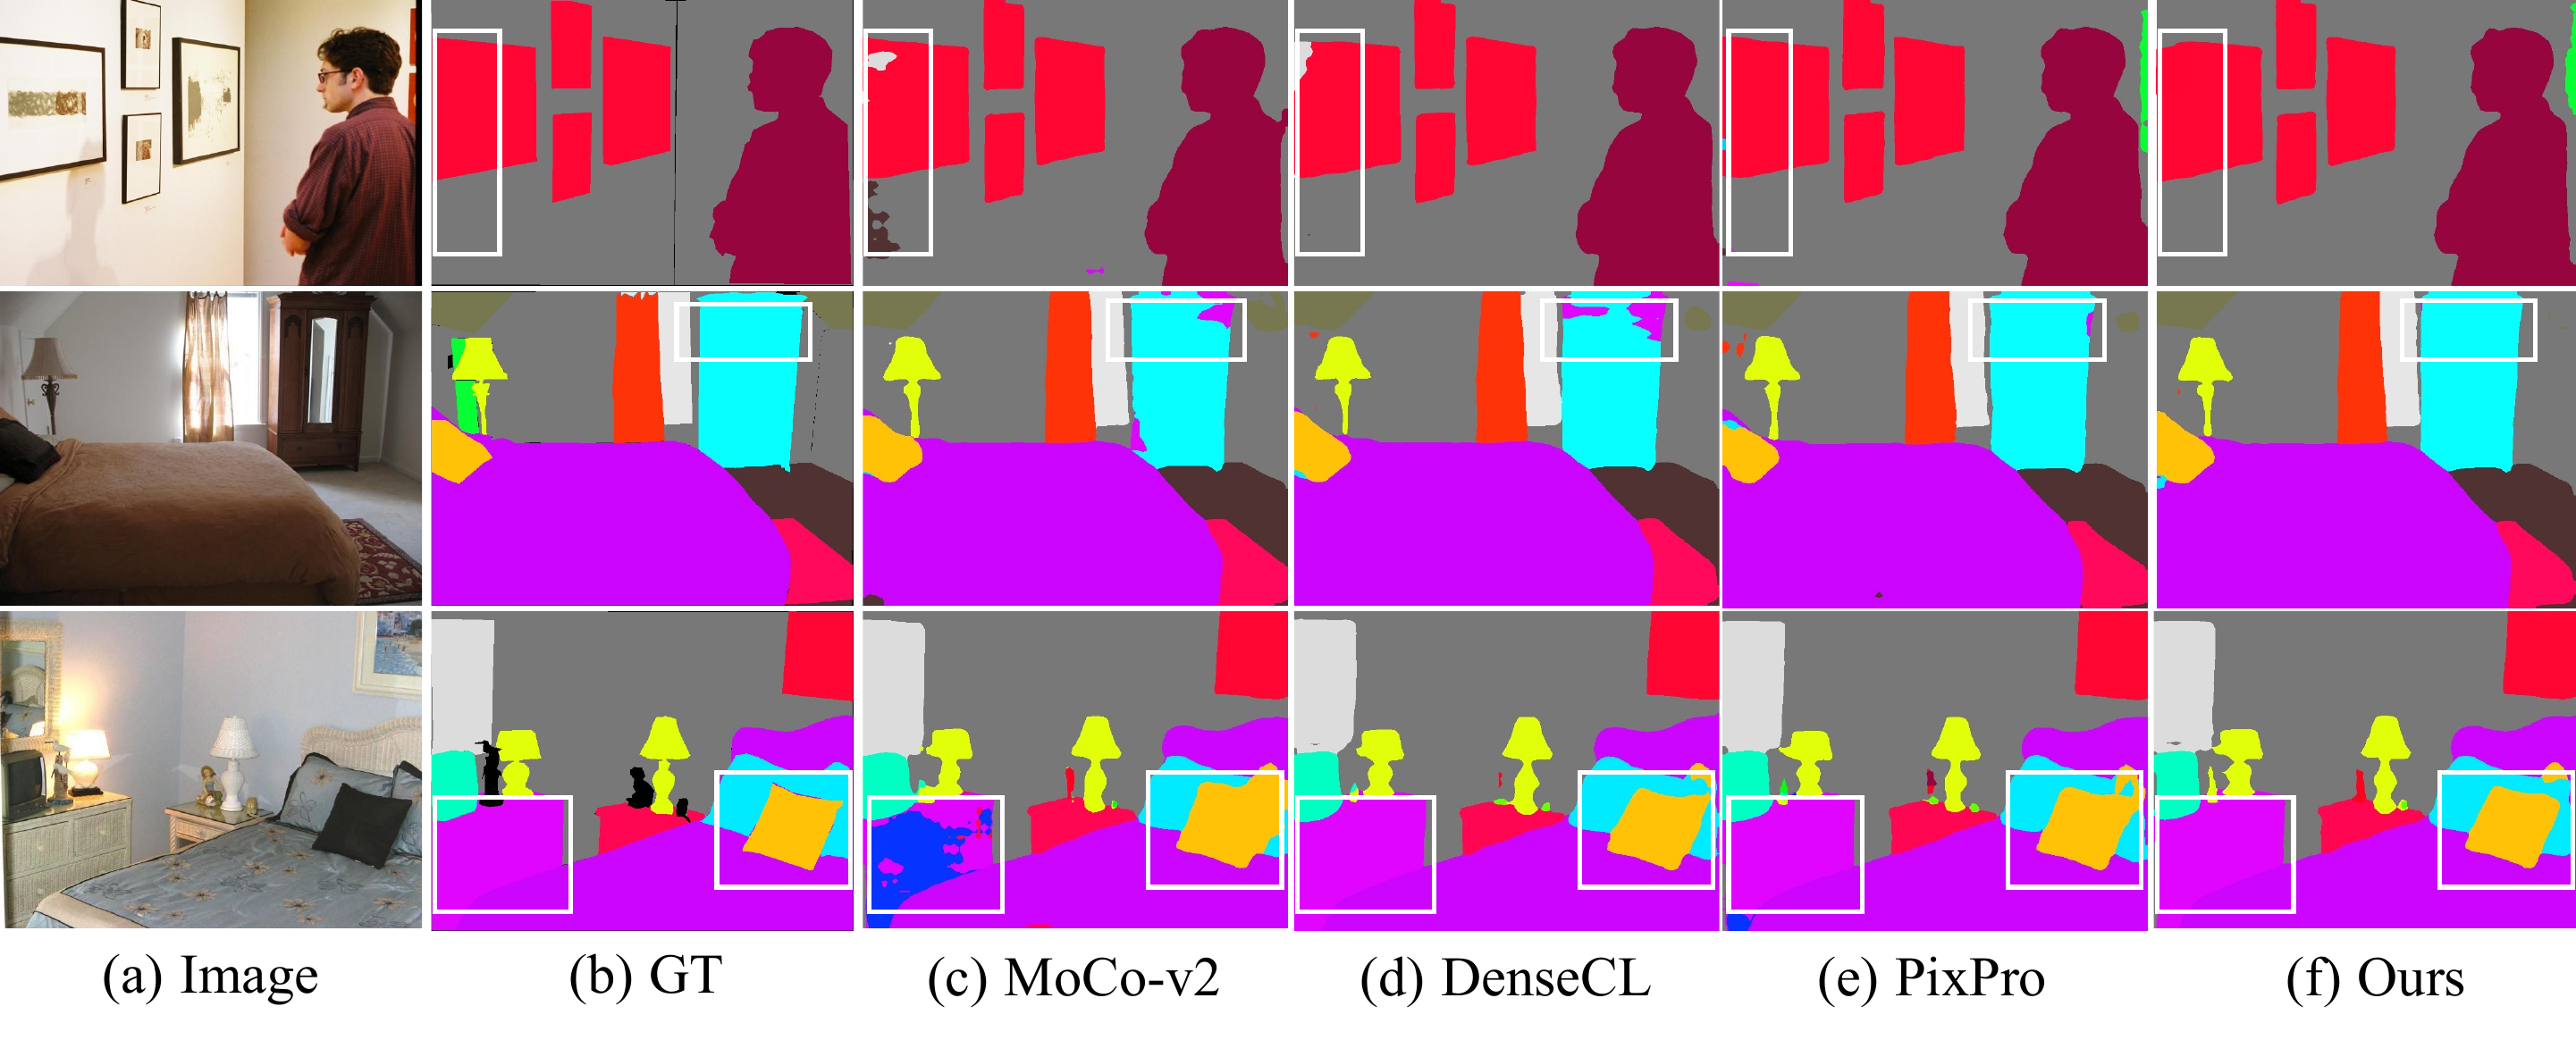}
        \caption{\textbf{Visualization results on ADE20K semantic segmentation.}
        (\textit{Best viewed in color.})}
    \label{fig:ade_seg} 
    \end{center}
\end{figure}
\begin{figure}[h]
    \begin{center}
        \includegraphics[scale=0.45]{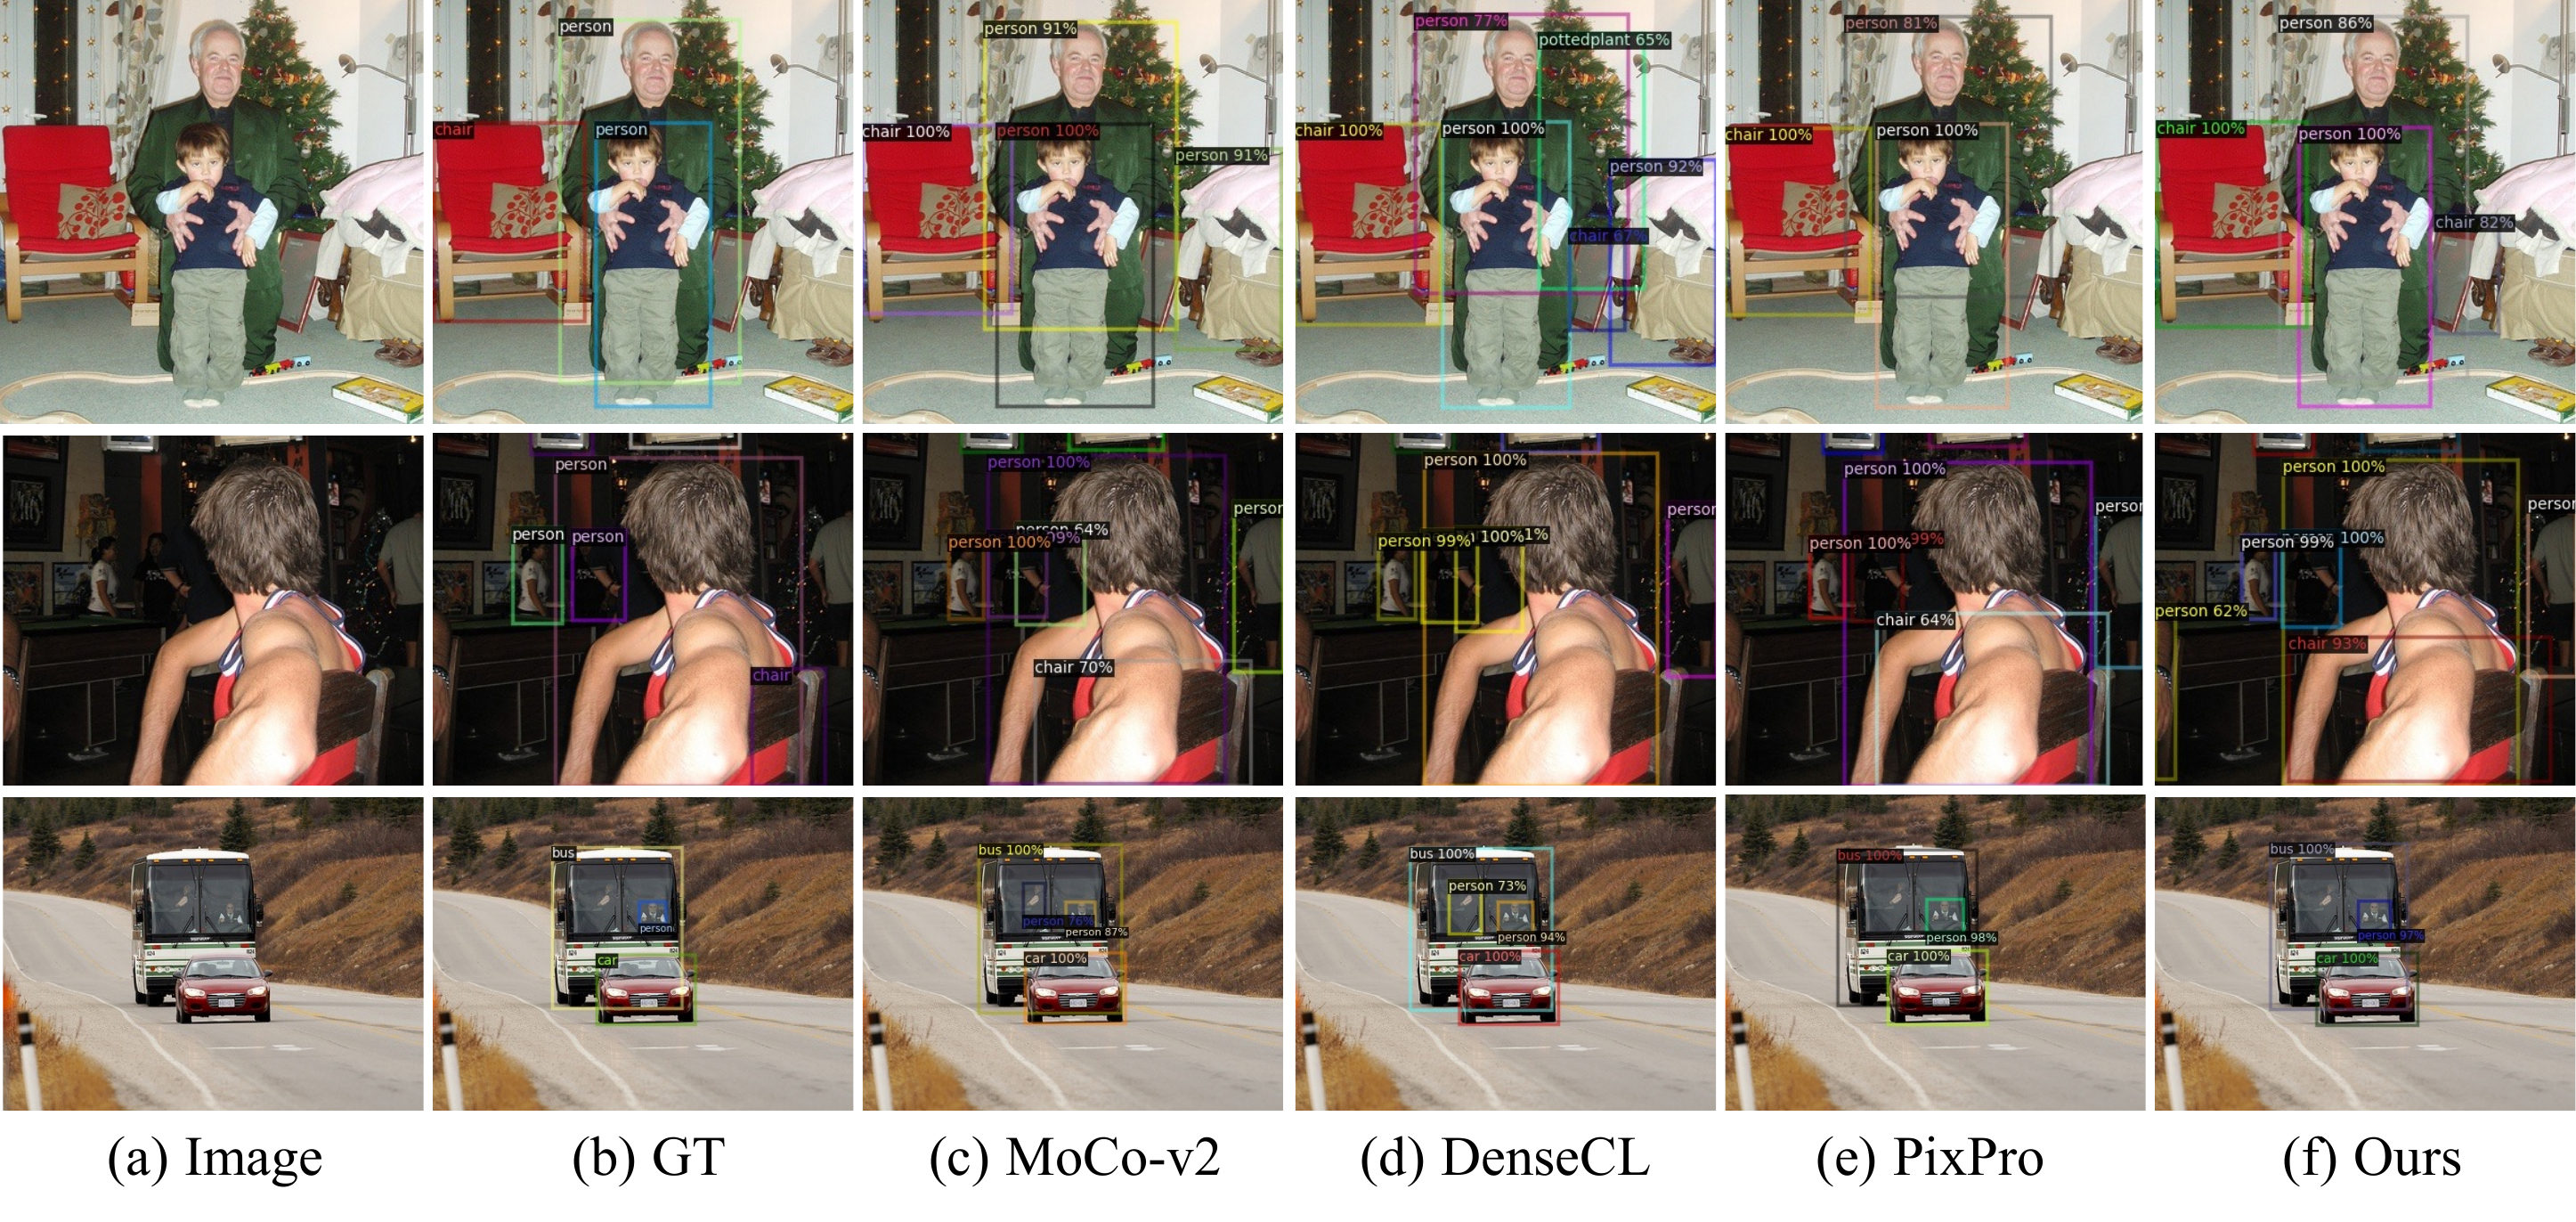}
        \caption{\textbf{Visualization results on PASCAL VOC object detection.}
        (\textit{Best viewed in color.})}
    \label{fig:voc_det} 
    \end{center}
\end{figure}
\begin{figure}[h]
    \begin{center}
        \includegraphics[scale=0.45]{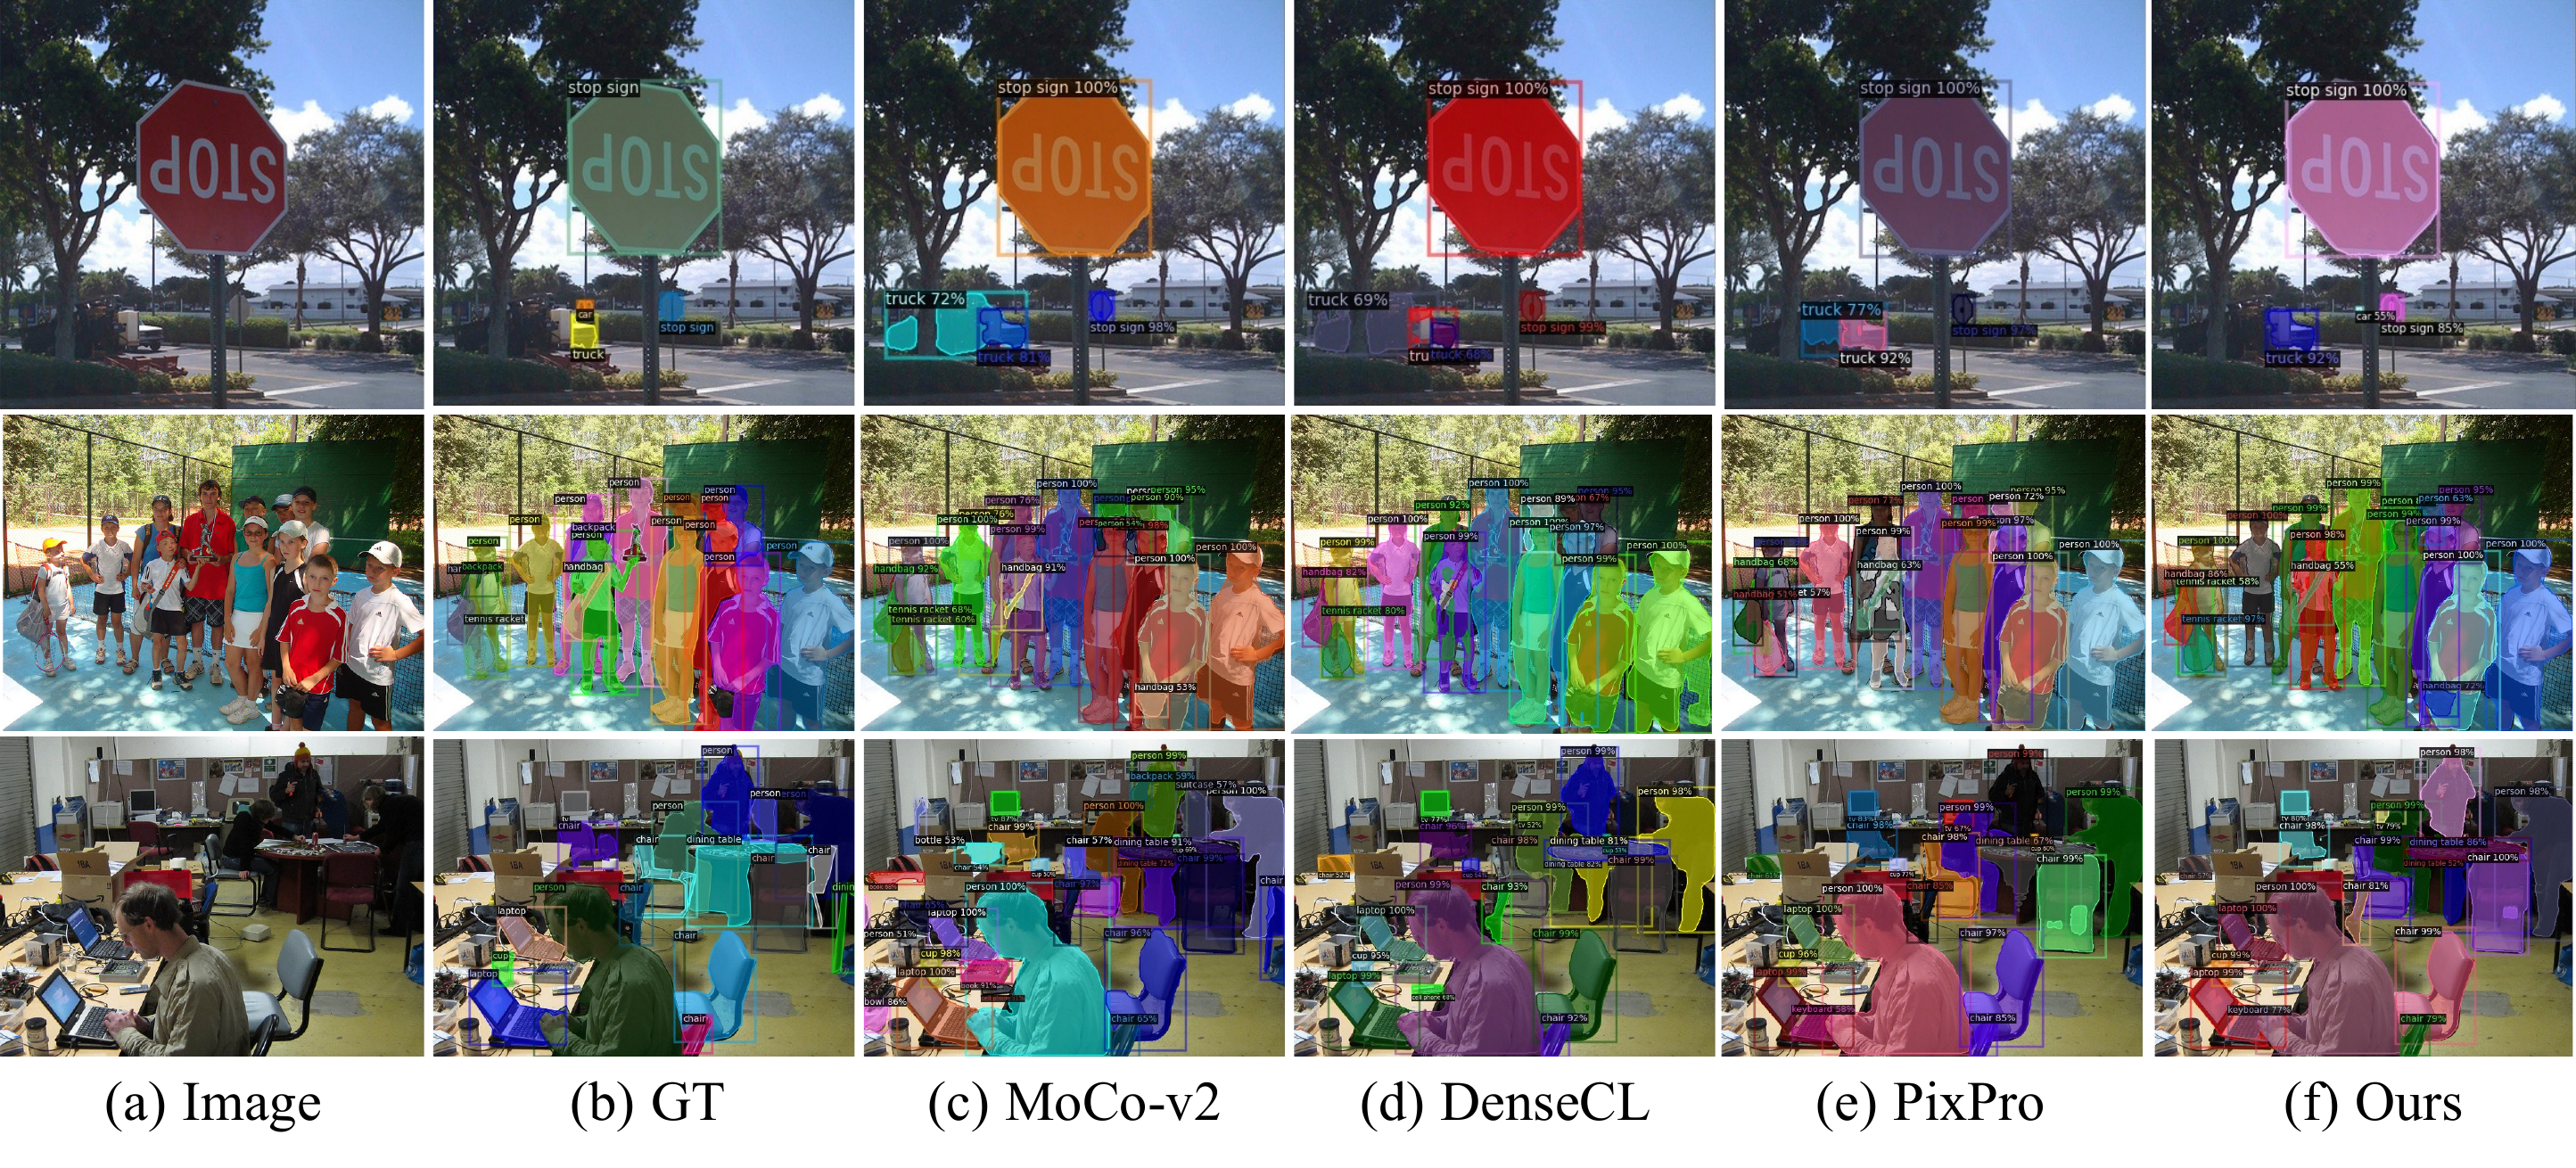}
        \caption{\textbf{Visualization results on COCO object detection and instance segmentation.}
        (\textit{Best viewed in color.})}
    \label{fig:coco_ins} 
    \end{center}
\end{figure}
\begin{figure}[h]
    \begin{center}
        \includegraphics[scale=0.45]{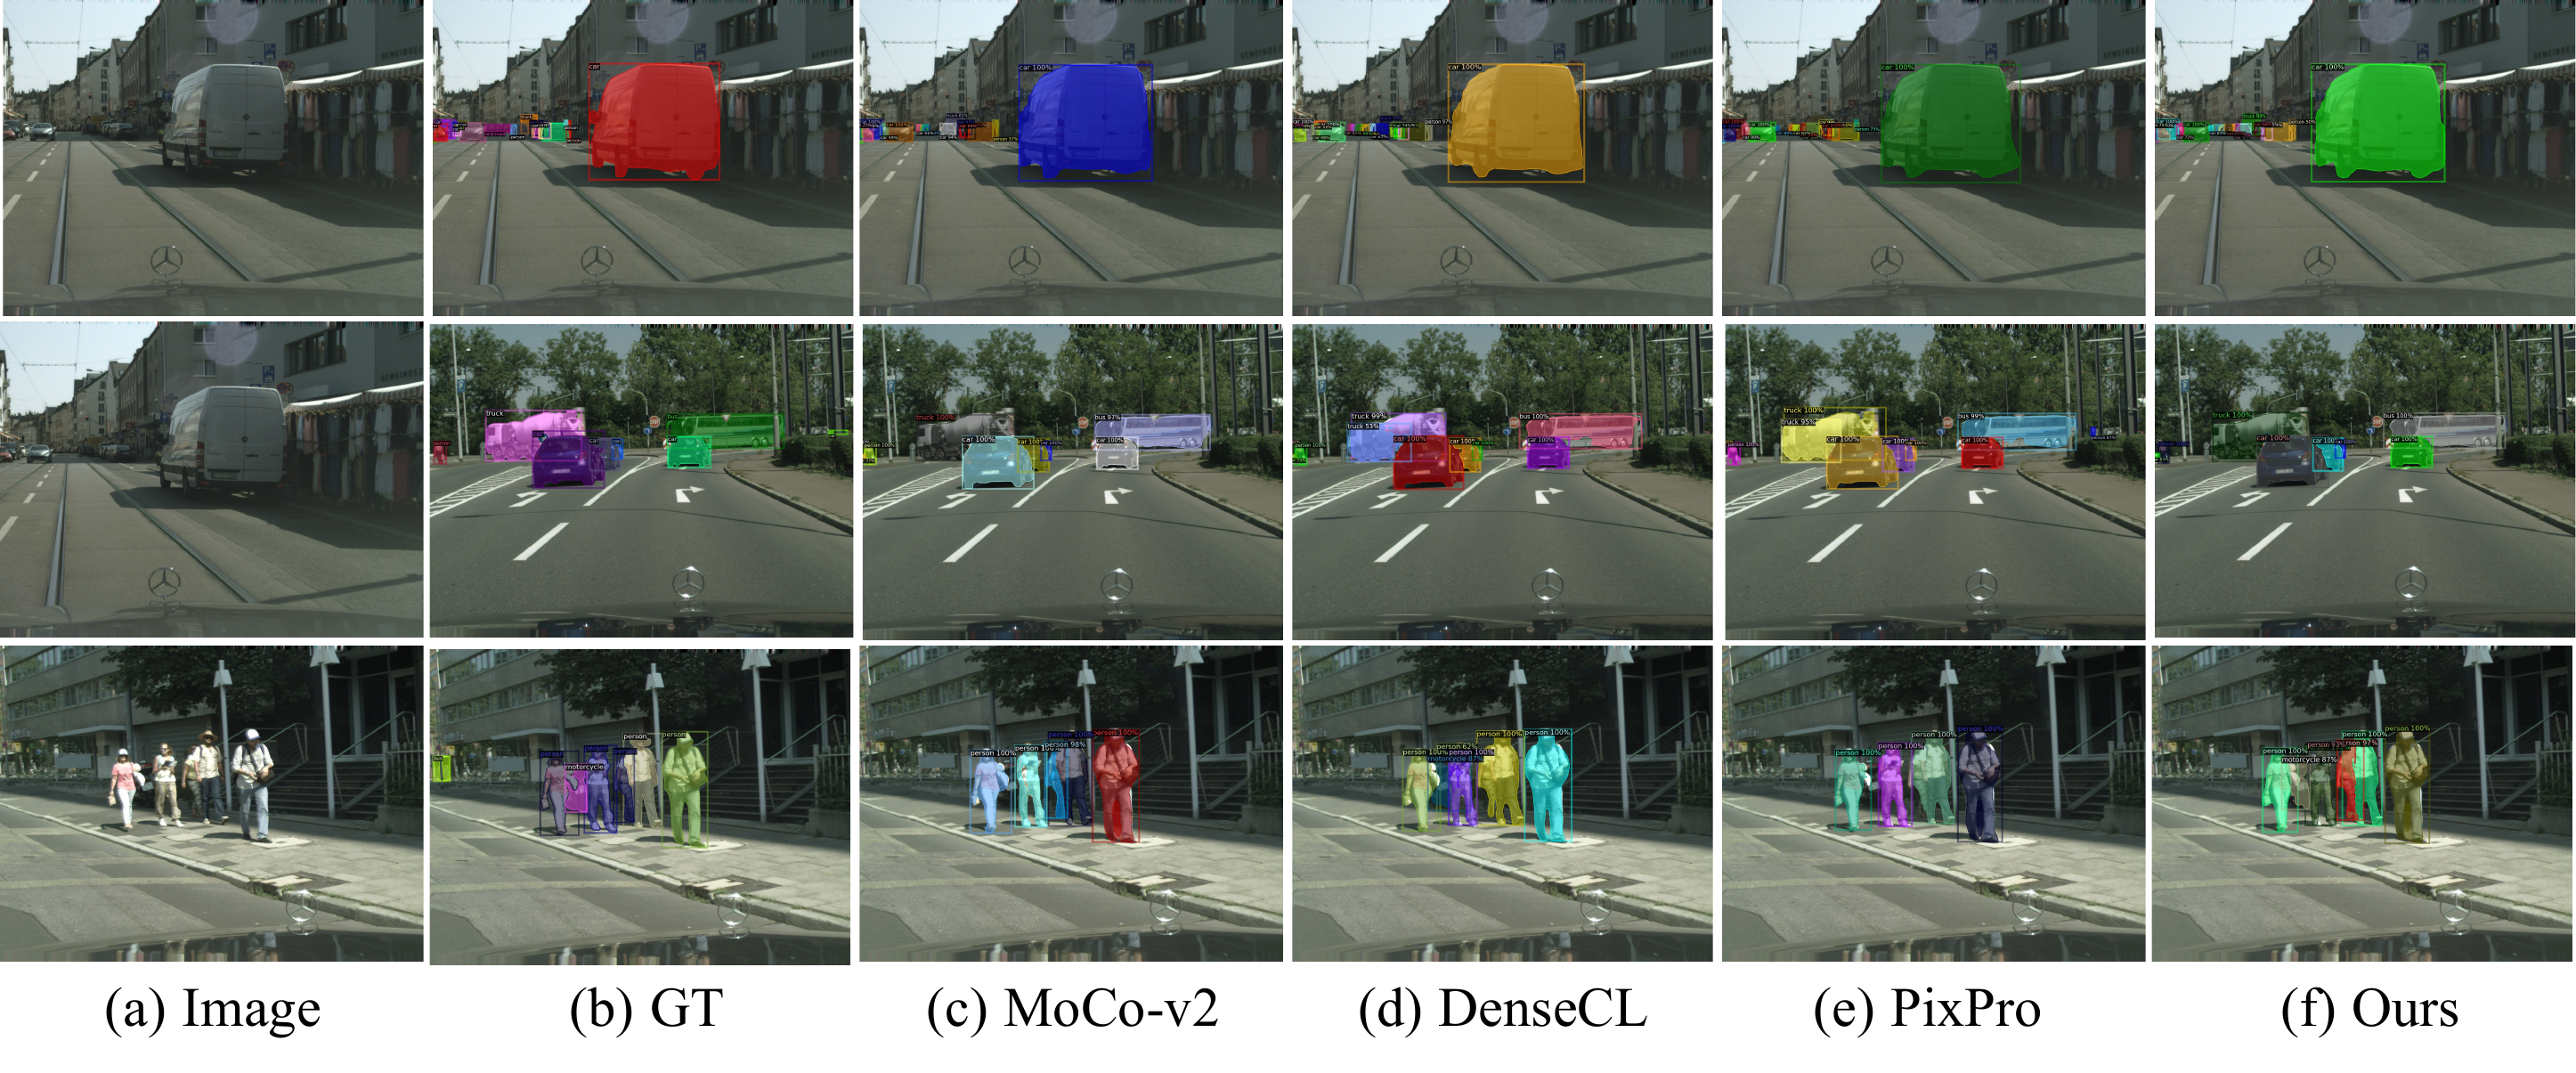}
        \caption{\textbf{Visualization results on Cityscapes instance segmentation.}
        (\textit{Best viewed in color.})}
    \label{fig:citys_ins} 
    \end{center}
\end{figure}
